# Supplementary material for: Sampling Algorithms for Butterfly Counting on Temporal Bipartite Graphs
Source: arXiv:2310.11886 source file (2023-10-18)
Supplement: Supplementary file 1 [file 7-appendix.tex]

\appendix

\section{Additional Experiments}
